# Supplementary material for: Differentially Private Exploration in Reinforcement Learning with Linear Representation
Source: arXiv:2112.01585 source file (2021-12-07)
Supplement: Supplementary file 1 [file 6appendix.tex]

%! TEX root = main.tex
